# Supplementary material for: Towards Automatic Parsing of Structured Visual Content through the Use of Synthetic Data
Source: arXiv:2204.14136 source file (2022-04-29)
Supplement: Supplementary file 1 [file 7_appendix.tex]

\begin{table}[!t]

\caption{Isomorphic Error on Synthetic Testset}
\label{iso_error_synthetic}
\centering
        \begin{tabular}{c||c|c|c|c|c}
        \hline
        \bfseries Structure & \bfseries Dir. & \bfseries Norm. & \bfseries Std. & \bfseries Mean & \bfseries [Min,Max]\\
        \hline\hline
        Full Graph &\cmark & \xmark  & 1.930   & 2.025 & [0,13]  \\
         &\xmark & \xmark   & 1.170  & 1.699 & [0,11]  \\
        %  \hline
         &\cmark & \cmark & 0.134  & 0.132 & [0,0.833]\\
         &\xmark & \cmark & 0.081  & 0.115 & [0,0.833]\\
        \hline
        %  \hline
        \hline
        Nodes && \xmark & 0.126   & 0.351 & [0,2]  \\
                %  \hline
        & & \cmark & 0.016  &  0.0479 & [0,0.5]\\
        \hline
        \hline
              Edges & \cmark & \xmark & 1.805   & 1.853 & [0,12]  \\
             & \xmark & \xmark & 1.045   & 1.484 & [0,9]  \\
            %  \hline
            & \cmark & \cmark   & 0.287  & 0.281 & [0,3]\\
             & \xmark & \cmark & 0.168  &  0.244 & [0,3]\\
        \hline
        \end{tabular}
\end{table}

\begin{table}[!t]

\caption{Isomorphic Error on Adjusted Synthetic Testset}
\label{iso_error_adjusted_synthetic}
\centering
        \begin{tabular}{c||c|c|c|c|c}
        \hline
        \bfseries Structure & \bfseries Dir. & \bfseries Norm. & \bfseries Std. & \bfseries Mean & \bfseries [Min,Max]\\
        \hline\hline
        Full Graph &\cmark & \xmark  & 0.645 & 0.863 & [0,3] \\
         &\xmark & \xmark   & 0.419 & 0.752 & [0,3] \\
        %  \hline
         &\cmark & \cmark &  0.043 & 0.057 & [0.0,0.2] \\
         &\xmark & \cmark & 0.03 & 0.053 & [0.0,0.2] \\
        \hline
        %  \hline
        \hline
        Nodes && \xmark &  0.065 & 0.246 & [0,1]\\
                %  \hline
        & & \cmark & 0.009 & 0.035 & [0.0,0.143]\\
        \hline
        \hline
              Edges & \cmark & \xmark & 0.581 & 0.872 & [0,3] \\
             & \xmark & \xmark & 0.355 & 0.743 & [0,3]\\
            %  \hline
            & \cmark & \cmark   & 0.1 & 0.163 & [0.0,0.667]\\
             & \xmark & \cmark & 0.068 & 0.152 & [0.0,0.667]\\
        \hline
        \end{tabular}
\end{table}
    
\begin{table}[!t]

\caption{Isomorphic Error on Disknet Testset}
\label{iso_error_disknet}
\centering
        \begin{tabular}{c||c|c|c|c|c}
        \hline
        \bfseries Structure & \bfseries Dir. & \bfseries Norm. & \bfseries Std. & \bfseries Mean & \bfseries [Min,Max]\\
        \hline\hline
        Full Graph &\cmark & \xmark  & 6.333 & 5.217 & [1,22] \\
         &\xmark & \xmark   & 5.75 & 4.746 & [1,21] \\
        %  \hline
         &\cmark & \cmark &  0.328 & 0.139 & [0.091,0.654] \\
         &\xmark & \cmark & 0.297 & 0.122 & [0.091,0.556] \\
        \hline
        %  \hline
        \hline
        Nodes && \xmark &  0.542 & 1.322 & [0,6]\\
                %  \hline
        & & \cmark & 0.037 & 0.076 & [0.0,0.273]\\
        \hline
        \hline
              Edges & \cmark & \xmark & 5.792 & 4.32 & [1,16]\\
             & \xmark & \xmark & 5.208 & 3.797 & [1,15]\\
            %  \hline
            & \cmark & \cmark   & 0.613 & 0.233 & [0.143,1.0]\\
             & \xmark & \cmark & 0.553 & 0.211 & [0.143,1.0]\\
        \hline
        \end{tabular}
\end{table}

\begin{table}[!t]

\caption{Isomorphic Error on Adjusted Disknet Testset}
\label{iso_error_adjusted_disknet}
\centering
        \begin{tabular}{c||c|c|c|c|c}
        \hline
        \bfseries Structure & \bfseries Dir. & \bfseries Norm. & \bfseries Std. & \bfseries Mean & \bfseries [Min,Max]\\
        \hline\hline
        Full Graph &\cmark & \xmark  & 5.059 & 4.094 & [1,17] \\
         &\xmark & \xmark   & 4.471 & 3.5 & [1,13] \\
        %  \hline
         &\cmark & \cmark &  0.325 & 0.139 & [0.091,0.654]\\
         &\xmark & \cmark & 0.291 & 0.123 & [0.091,0.556]\\
        \hline
        %  \hline
        \hline
        Nodes && \xmark &  0.235 & 0.73 & [0,3]\\
                %  \hline
        & & \cmark & 0.021 & 0.062 & [0.0,0.25]\\
        \hline
        \hline
              Edges & \cmark & \xmark & 4.824 & 3.714 & [1,16]\\
             & \xmark & \xmark & 4.235 & 3.078 & [1,12]\\
            %  \hline
            & \cmark & \cmark   & 0.622 & 0.226 & [0.2,1.0]\\
             & \xmark & \cmark & 0.558 & 0.213 & [0.2,1.0]\\
        \hline
        \end{tabular}
\end{table}

\begin{table}[!t]

\caption{OCR Error}
\label{ocr_error}
\centering
        \begin{tabular}{c||c|c|c}
        \hline
        \bfseries Dataset &\bfseries Std. & \bfseries Mean & \bfseries [Min,Max]\\
        \hline\hline
        Synthetic Testset & 0.423 & 0.429 & [0.0,13.0] \\
        Adjusted Synthetic Testset & 0.29 & 0.115 & [0.091,0.474] \\
        Disknet Testset & 0.254 & 0.214 & [0.039,0.692] \\
        Adjusted Disknet Testset & 0.2 & 0.187 & [0.039,0.692] \\

        \hline
        \end{tabular}
\end{table}
