# Supplementary material for: Towards Automatic Parsing of Structured Visual Content through the Use of Synthetic Data
Source: arXiv:2204.14136 source file (2022-04-29)
Supplement: Supplementary file 2 [file supplemental.tex]

% \documentclass[a4paper,conference,onecolumn]{IEEEtran}

% \usepackage{blindtext}
% \usepackage{graphicx}
% \usepackage{pifont}
% \usepackage{multicol}
% \usepackage{multirow}
% \usepackage{makecell}

% \title{Supplementary Material of Towards Automatic Parsing of Structured Visual Content through the Use of Synthetic Data}

% \author{Lukas Sch\"olch\IEEEauthorrefmark{1}, Jonas Steinh\"auser\IEEEauthorrefmark{1}, Maximilian Beichter\IEEEauthorrefmark{1}, Constantin Seibold\IEEEauthorrefmark{2}, Kailun Yang\IEEEauthorrefmark{2},\\Merlin Knaeble\IEEEauthorrefmark{2}, Thorsten Schwarz\IEEEauthorrefmark{2}, Alexander Maedche\IEEEauthorrefmark{2}, and Rainer Stiefelhagen\IEEEauthorrefmark{2}
% \\Karlsruhe Institute of Technology, Germany
% \\\IEEEauthorrefmark{1}equal contribution, {\tt\small \{firstname.lastname\}@student.kit.edu}, \IEEEauthorrefmark{2}{\tt\small \{firstname.lastname\}@kit.edu}
% }

% \begin{document}
% \maketitle

\section{Supplementary Material}

\subsection{Synthetic and Real Difficulties}

Our generation produces some diagrams which are ambiguous. These problems are intentionally not handled, since some of them may represent real situations or at least approximate them. Examples of this are shown in Fig \ref{fig:mergeArrows} and Fig \ref{fig:weightPositioning}.\\ 

Fig \ref{fig:mergeArrows}~(a) shows a generated diagram where two edges point to the same place of a node, which causes them to overlap. This case is graphically almost identical to merging edges as they exist in real images. An example of this is Fig \ref{fig:mergeArrows}~(b) from the Disknet dataset. This applies similarly to splitting edges.

\begin{figure*}
\centering
\begin{tabular}{cc}
    \includegraphics[width=0.45\linewidth,height=0.25\linewidth]{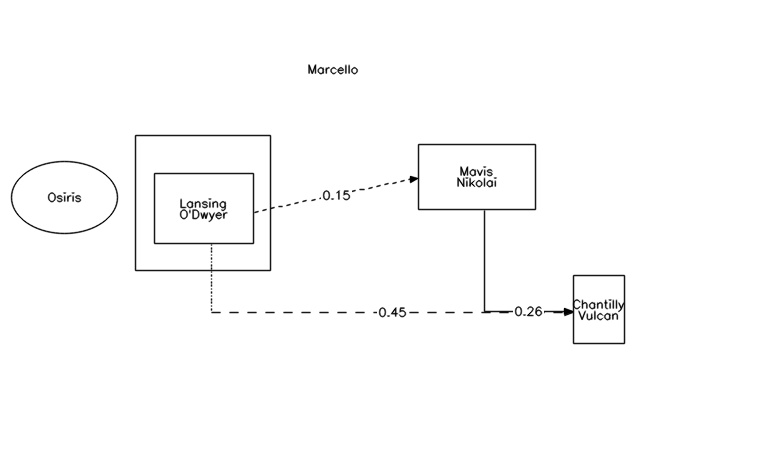}
    &
    \includegraphics[width=0.45\linewidth,height=0.25\linewidth]{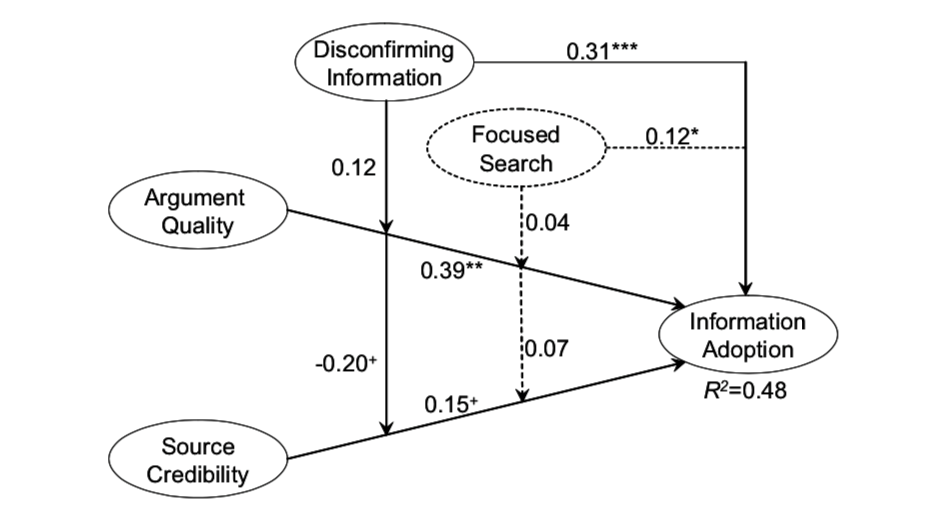}  \\
    \footnotesize{(a) Example of our generated dataset.} & 
    \footnotesize{(b) Example from the DISKNET dataset.}
\end{tabular}
\caption{Overlapping arrows can be interpreted as a merge.}
\label{fig:mergeArrows}
\end{figure*}

Fig \ref{fig:weightPositioning}~(a) shows a generated example where some edge weights have been placed in such a way that they lie over several edges. This leads to the fact that it is hardly possible to determine to which edge the weight belongs. Such an error also occurs quite often with overlapping edges. Fig \ref{fig:weightPositioning}~(b) shows a similar case in the Disknet dataset. In this case, it is also difficult to determine to which edge a weight belongs by looking at the individual weights.

\begin{figure*}[h]
\centering
\begin{tabular}{cc}
    \includegraphics[width=0.45\linewidth,height=0.25\linewidth]{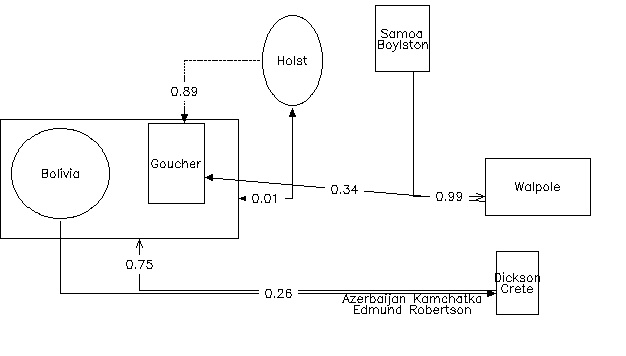}
    &
    \includegraphics[width=0.45\linewidth,height=0.25\linewidth]{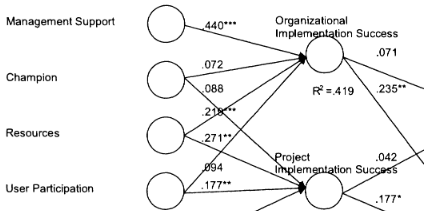}  \\
    \footnotesize{(a) Example of our generated dataset.} & 
    \footnotesize{(b) Example from the DISKNET dataset.}
\end{tabular}
\caption{Ambiguous positioning of edge weights exist in both synthetic and real data sets}
\label{fig:weightPositioning}
\end{figure*}

% \subsection{Error Measures Examples}

% \begin{figure}[h]
% \centering
% \begin{tabular}{cc}
%     \includegraphics[width=0.45\linewidth,height=0.3\linewidth]{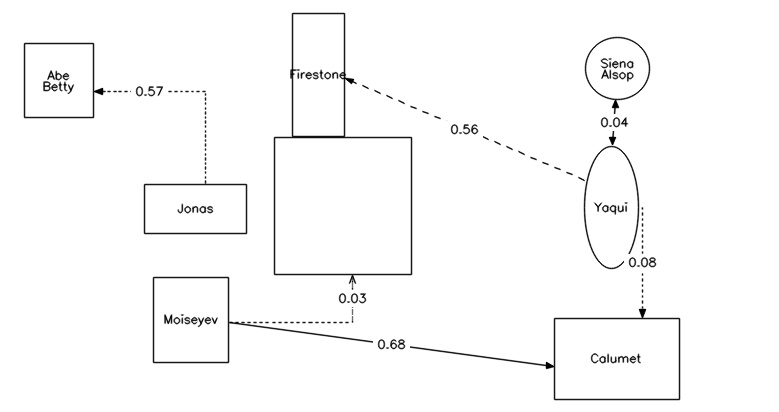}
%     &
%     \includegraphics[width=0.45\linewidth,height=0.3\linewidth]{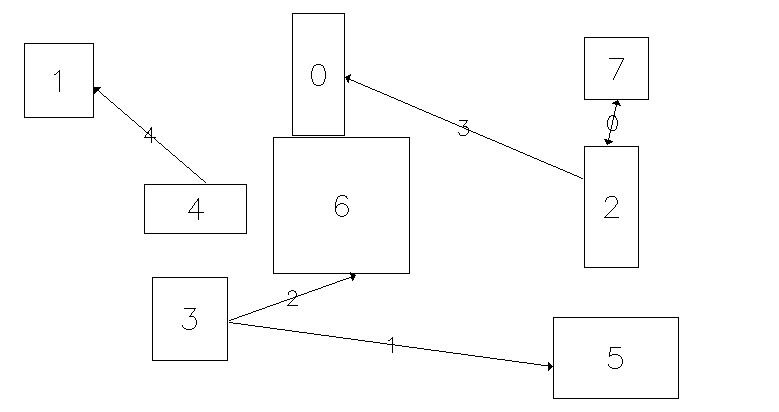}  \\
%     \footnotesize{(a) Example of our generated dataset.} & 
%     \footnotesize{(b) Graphical reconstruction of the detected structure of the graph.}
% \end{tabular}
% \caption{A synthetic graph with a graphical representation of the recognized structure. Thereby graphical details, like the shape of a node, are no longer considered. The respective elements are drawn with their corresponding ID. It can be seen that the edge from node 2 to 5 is lost in the recognition. Consequently, the \textit{IsomorphicError} is 1 and the \textit{NormIsomorphicError} $1/14$.}
% \label{fig:reconstruction}
% \end{figure}

% \begin{figure}[h]
% \centering
% \begin{tabular}{cc}
%     \includegraphics[width=0.45\linewidth,height=0.3\linewidth]{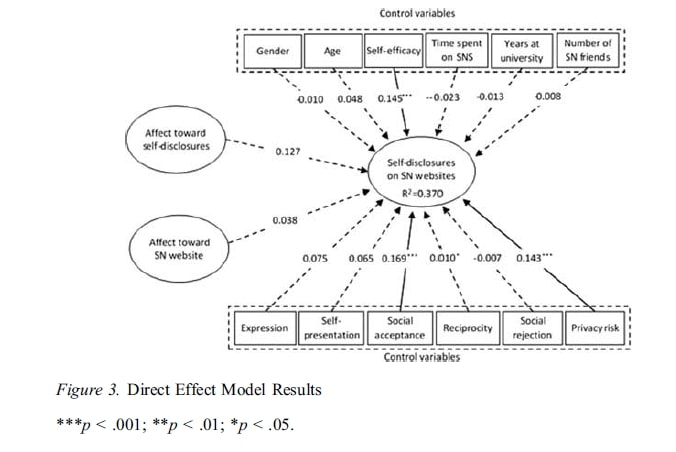}
%     &
%     \includegraphics[width=0.45\linewidth,height=0.3\linewidth]{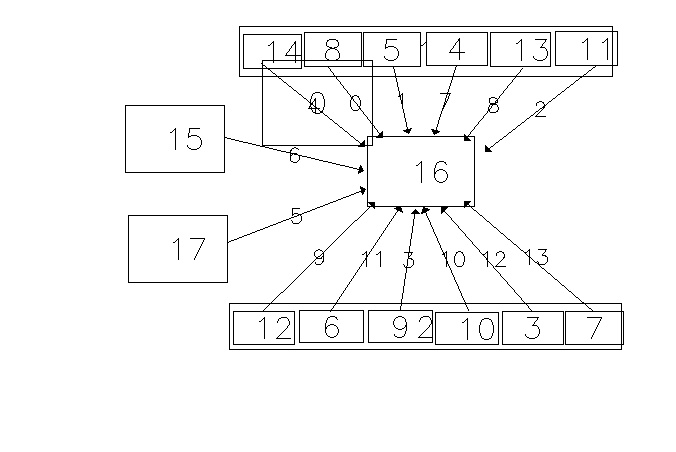}  \\
%     \footnotesize{(a) Example from the DISKNET dataset.} & 
%     \footnotesize{(b) Graphical reconstruction of the detected structure from the object detection.}
% \end{tabular}
% \caption{.}
% \label{fig:disknet_big}
% \end{figure}

\subsection{Examples of processing real world SVCs}
The following images show the original SVCs from the DISKNET dataset, their reconstruction from the object detection and their manual reconstruction from the graph representation. While there are some minor errors, the overall process works very well and the original SVC is nearly perfectly transferred into a textual and machine readable graph representation.

Fig \ref{fig:DISKNET1-original} shows a SVC from the DISKNET dataset. Fig \ref{fig:DISKNET1-reconstruction}~(a) shows a reconstruction from the information we got from the object detection. Here we only use positional and class information to draw the reconstruction. Fig \ref{fig:DISKNET1-reconstruction}~(b) shows a manual reconstruction from the graph representation. Here we do not have any positional information stored but show the graph layout in a similar layout to the original SVC to better compare errors. This visualization is only done here to showcase the textual graph representation. 

It is visible that there is one edge missing as it was not detected in the object detection step. Other than that the detection and reconstructed worked correctly. Therefore the absolute IsoError is 1 and the relative IsoError is 1/13.
The text recognition on the other hand did not work as good in this image as it did in other images. Anyhow, this is not a main focus in our work as the OCR method can be easily swapped for a different one.

\begin{figure}[h]
    \centering
    \includegraphics[width=0.9\linewidth,height=0.5\linewidth]{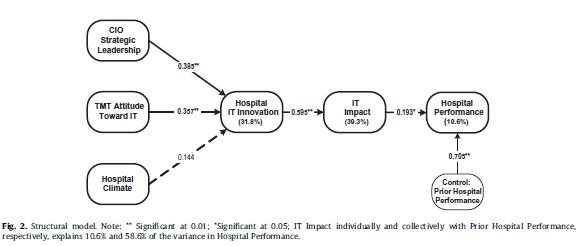}
    \caption{Original SVC from DISKNET}
    \label{fig:DISKNET1-original}
\end{figure}

\begin{figure}[h]
\centering
\begin{tabular}{c}
    \includegraphics[width=0.9\linewidth,height=0.5\linewidth]{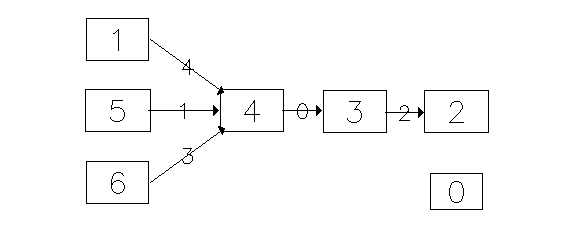}
    \\
    \includegraphics[width=0.9\linewidth,height=0.5\linewidth]{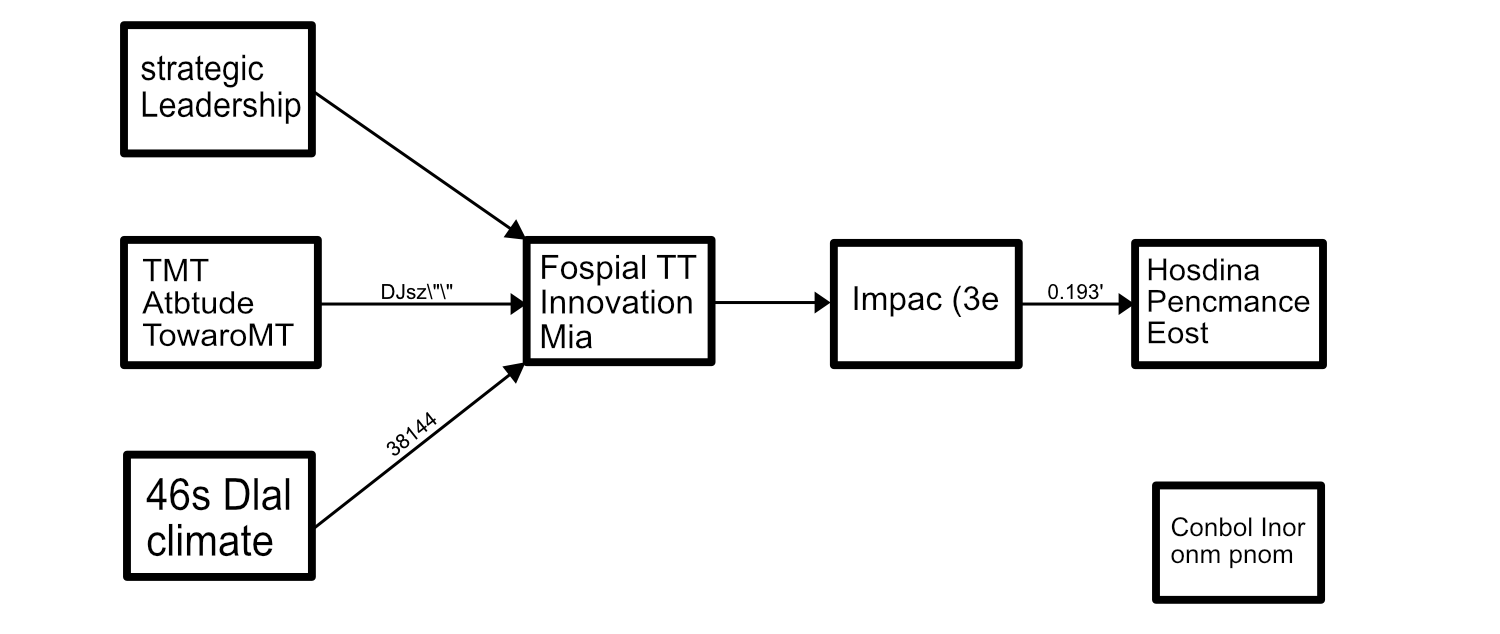}\\
    \footnotesize{(a) Reconstruction from the object detection} & 
    \footnotesize{(b) Reconstruction from the graph representation}
\end{tabular}
\caption{Reconstructions of the original SVC in Fig \ref{fig:DISKNET1-original}}
\label{fig:DISKNET1-reconstruction}
\end{figure}

% \newpage

Fig \ref{fig:DISKNET2-original} shows a SVC from the DISKNET dataset. Fig \ref{fig:DISKNET2-reconstruction}~(a) shows a reconstruction from the information we got from the object detection. Here we only use positional and class information to draw the reconstruction. Fig \ref{fig:DISKNET2-reconstruction}~(b) shows a manual reconstruction from the graph representation. Here we do not have any positional information stored but show the graph layout in a similar layout to the original SVC to better compare errors. This visualization is only done here to showcase the textual graph representation.

It is visible that there is one additional node detected that is not supposed to be there. Unfortunately, this leads to another error in the graph reconstruction, where the correct detected edge 4 gets assigned to the wrongly detected node 0. Apart from this, all other detections and reconstructions worked correctly. This is a good result, also showing that the tight layout of the groupings were recognized correctly.
This leads to an absolute IsoError of 3 and a relative IsoError of 3/31. 
The error is calculated by the fact that there is one node too much and an edge was assigned incorrectly. The incorrectly assigned edge is counted twice because an edge appears in a place where it should not be and is missing in its actual place.
Again, the text is not detected optimally.

\begin{figure*}[h]
    \centering
    \includegraphics[width=0.45\linewidth]{IEEEconf_ICPR2020/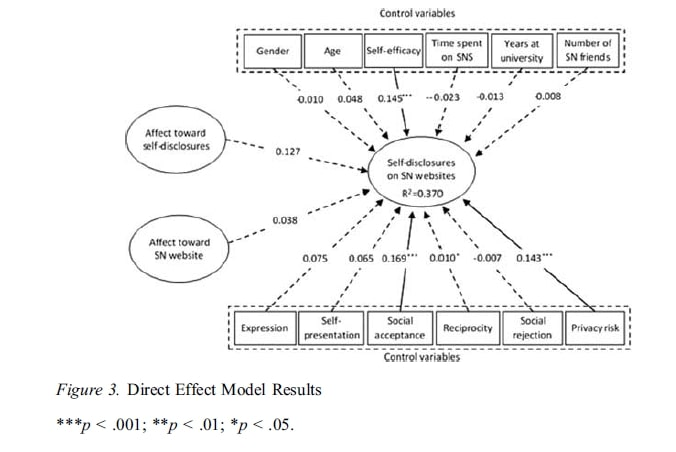}
    \caption{Original SVC from DISKNET}
    \label{fig:DISKNET2-original}
\end{figure*}

\begin{figure*}[h]
% \centering
\begin{tabular}{cc}
    \includegraphics[width=0.45\linewidth]{IEEEconf_ICPR2020/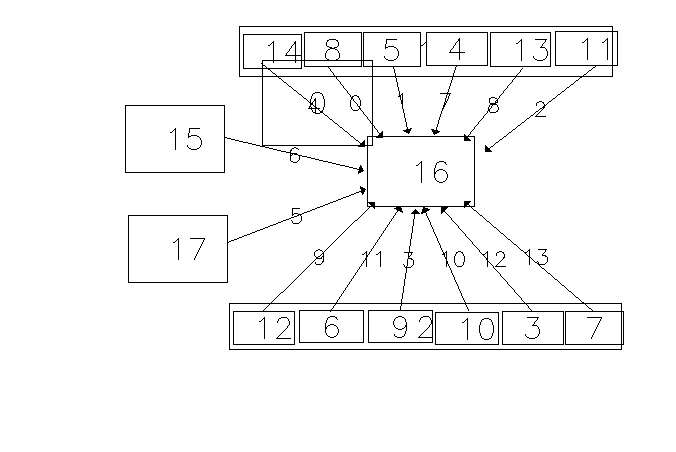}
    &
    \includegraphics[width=0.45\linewidth]{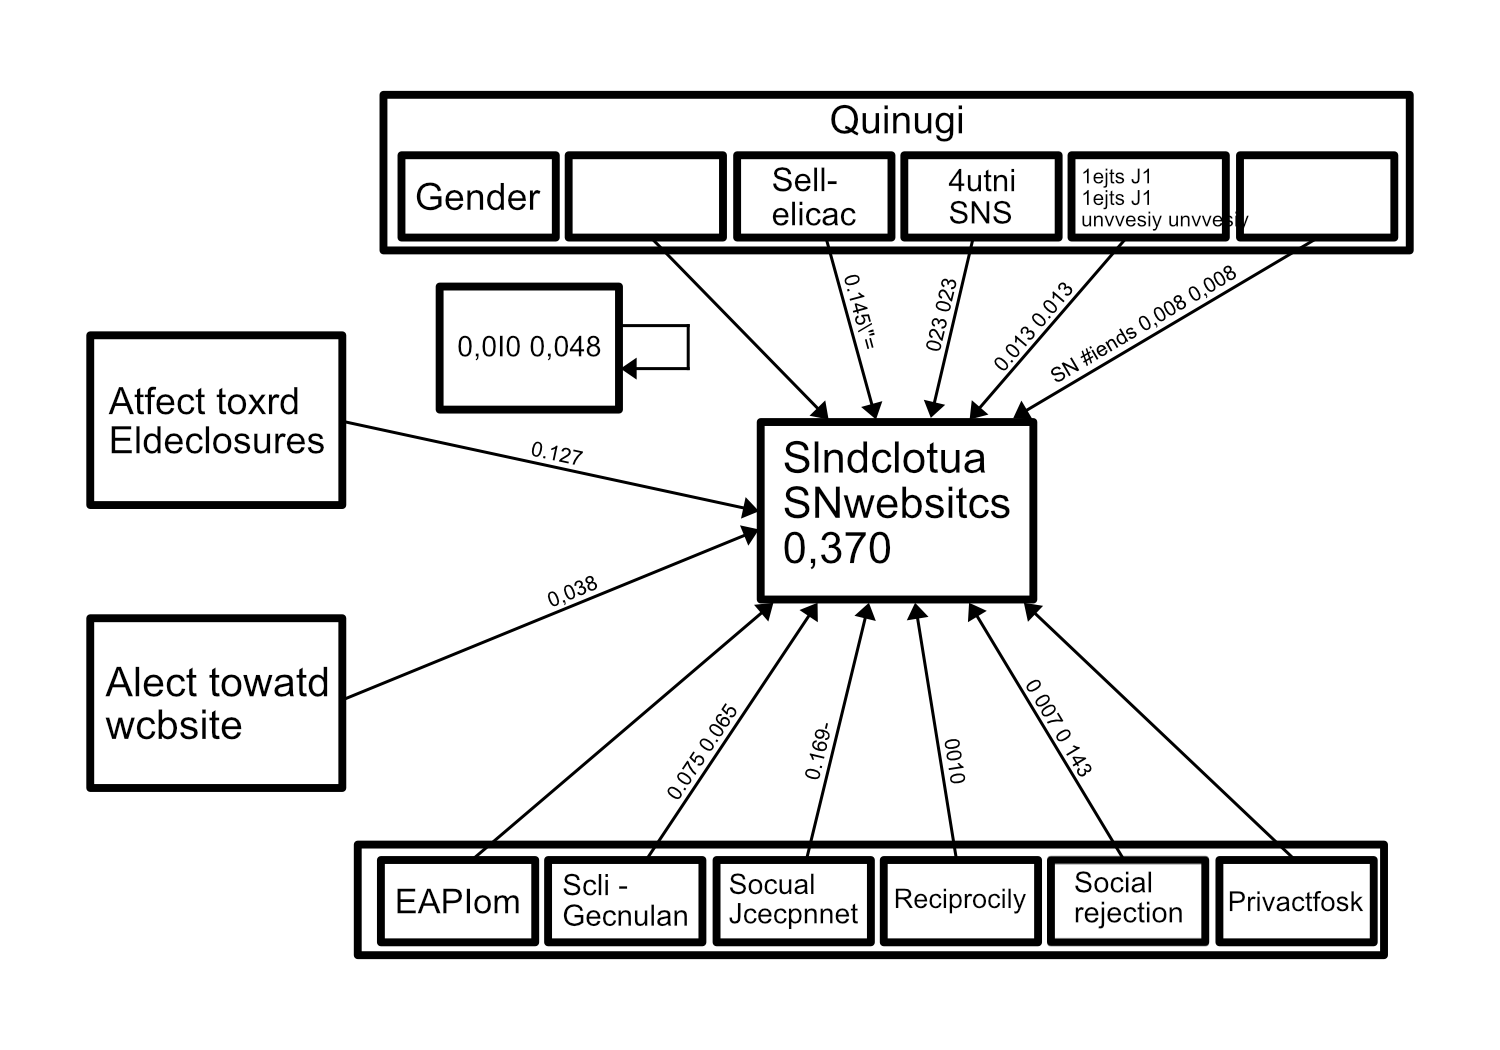}\\
    \footnotesize{(a) Reconstruction from the object detection} & 
    \footnotesize{(b) Reconstruction from the graph representation}
\end{tabular}
\caption{Reconstructions of the original SVC in Fig \ref{fig:DISKNET2-original}}
\label{fig:DISKNET2-reconstruction}
\end{figure*}

% \end{document}
